# Supplementary material for: Leveraging Class Hierarchies with Metric-Guided Prototype Learning
Source: arXiv:2007.03047 source file (2021-11-29)
Supplement: Supplementary file 2 [file appendix_standalone.tex]

\documentclass{article}

\usepackage{neurips_2020}

% to compile a preprint version, e.g., for submission to arXiv, add add the
% [preprint] option:

\usepackage[utf8]{inputenc} % allow utf-8 input
\usepackage[T1]{fontenc}    % use 8-bit T1 fonts
\usepackage{hyperref}       % hyperlinks
\usepackage{url}            % simple URL typesetting
\usepackage{booktabs}       % professional-quality tables
\usepackage{amsfonts}       % blackboard math symbols
\usepackage{nicefrac}       % compact symbols for 1/2, etc.
\usepackage{microtype}      % microtypography
\usepackage{listings}

\usepackage{amsmath}
\usepackage{amssymb}
\usepackage{inputenc, caption, graphicx, color}

\usepackage{balance}
\usepackage[normalem]{ulem}
\usepackage{multicol}
\usepackage{multirow}
\usepackage{placeins}
\usepackage{booktabs}
\usepackage{subcaption}
\usepackage{style}
\usepackage{tikz}
\usepackage[edges]{forest}
\usepackage{flexisym}
\usetikzlibrary{shapes}

\usepackage{booktabs}

%distrotion-based metric loss

\newcommand{\killpunct}[1]{}%necessary to remove dot after punctuation marks in citations' title. dirty dirty hack https://tex.stackexchange.com/questions/181130/remove-question-mark-following-period-for-reference-title-in-pdf-using-vancouve/181298#181298

\usepackage{xcolor}

\colorlet{punct}{red!60!black}
\definecolor{background}{HTML}{EEEEEE}
\definecolor{delim}{RGB}{20,105,176}
\colorlet{numb}{magenta!60!black}

\lstdefinelanguage{json}{
    basicstyle=\scriptsize\ttfamily,
    numberstyle=\scriptsize,
    stepnumber=1,
    numbersep=8pt,
    showstringspaces=false,
    breaklines=true,
    frame=lines,
    %backgroundcolor=\color{background},
    literate=
     *{0}{{{\color{numb}0}}}{1}
      {1}{{{\color{numb}1}}}{1}
      {2}{{{\color{numb}2}}}{1}
      {3}{{{\color{numb}3}}}{1}
      {4}{{{\color{numb}4}}}{1}
      {5}{{{\color{numb}5}}}{1}
      {6}{{{\color{numb}6}}}{1}
      {7}{{{\color{numb}7}}}{1}
      {8}{{{\color{numb}8}}}{1}
      {9}{{{\color{numb}9}}}{1}
      {:}{{{\color{punct}{:}}}}{1}
      {,}{{{\color{punct}{,}}}}{1}
      {\{}{{{\color{delim}{\{}}}}{1}
      {\}}{{{\color{delim}{\}}}}}{1}
      {[}{{{\color{delim}{[}}}}{1}
      {]}{{{\color{delim}{]}}}}{1},
}

\title{Supplementary Material for:\\ Metric-Guided Prototype Learning}

% The \author macro works with any number of authors. There are two commands
% used to separate the names and addresses of multiple authors: \And and \AND.
%
% Using \And between authors leaves it to LaTeX to determine where to break the
% lines. Using \AND forces a line break at that point. So, if LaTeX puts 3 of 4
% authors names on the first line, and the last on the second line, try using
% \AND instead of \And before the third author name.

\author{%
Vivien Sainte Fare Garnot\thanks{vivien.sainte-fare-garnot@ign.fr} , Loic Landrieu \\
   LASTIG, ENSG, IGN\\
   Univ Gustave Eiffel\\
  F-94160 Saint-Mande, France \\

  % \AND
  % Coauthor \\
  % Affiliation \\
  % Address \\
  % \texttt{email} \\
  % \And
  % Coauthor \\
  % Affiliation \\
  % Address \\
  % \texttt{email} \\
  % \And
  % Coauthor \\
  % Affiliation \\
  % Address \\
  % \texttt{email} \\
}

\begin{document}

\maketitle
\setcounter{figure}{2}   
\input{appendixv2}

\end{document}
